# Supplementary material for: A critical examination of robustness and generalizability of machine learning prediction of materials properties
Source: arXiv:2210.13597 source file (2022-10-24)
Supplement: Supplementary file 1 [file supplemental_information.pdf]

# Supplemental information for: A critical examination of robustness and generalizability of machine learning prediction of materials properties

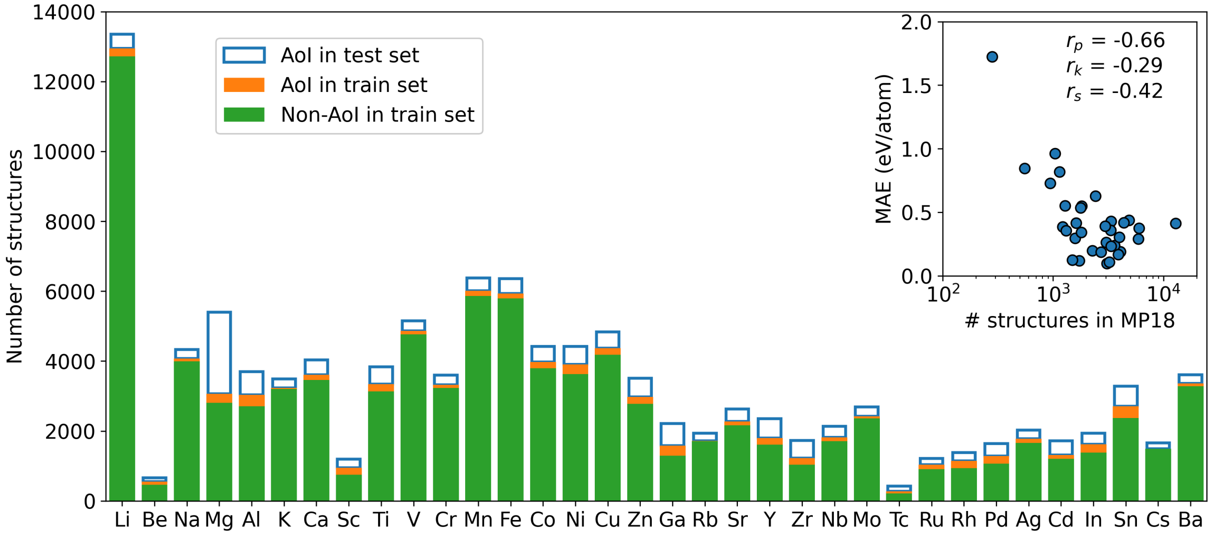


FIG. S1. Number of structures that contain a given element of interest. The inset shows the correlation between the MAE in the alloy test set and the number of structures in the whole MP18 training set for each metallic element. $r_p$, $r_s$ and $r_k$ are respectively the Pearson, Spearman , and Kendall correlation coefficients.

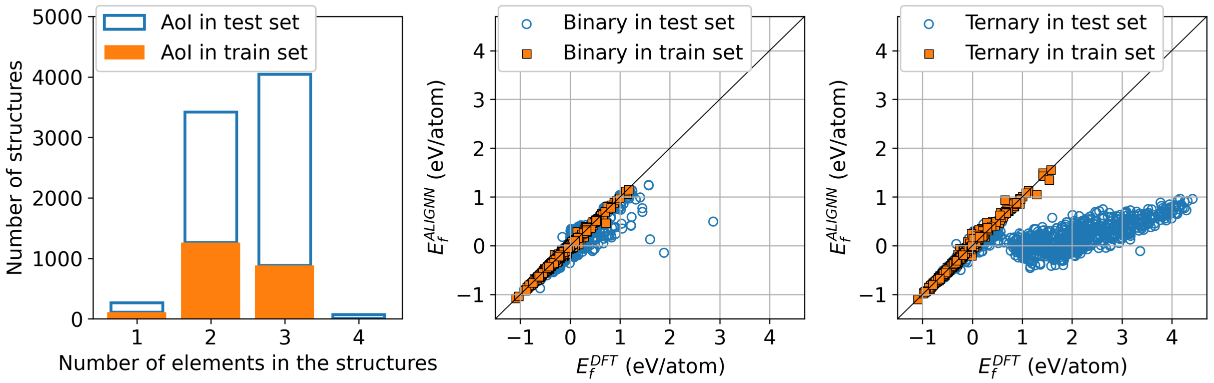


FIG. S2. Number of structures versus number of elements contained in the structures, and the ALIGNN performance on binary and ternary alloys of interest (AoI).

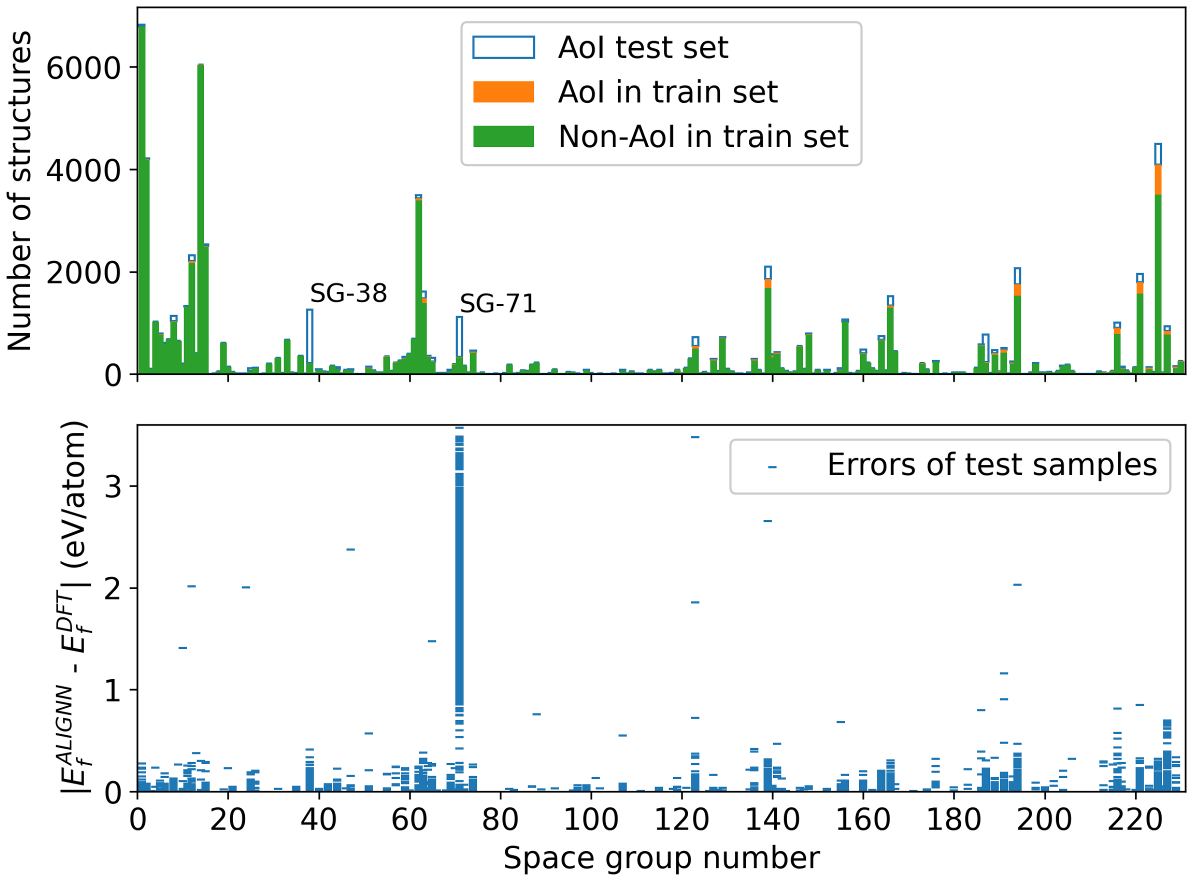


FIG. S3. Upper panel: number of structures as a function of space group number. Lower panel: distribution of prediction errors versus space group number for the AoI test data.

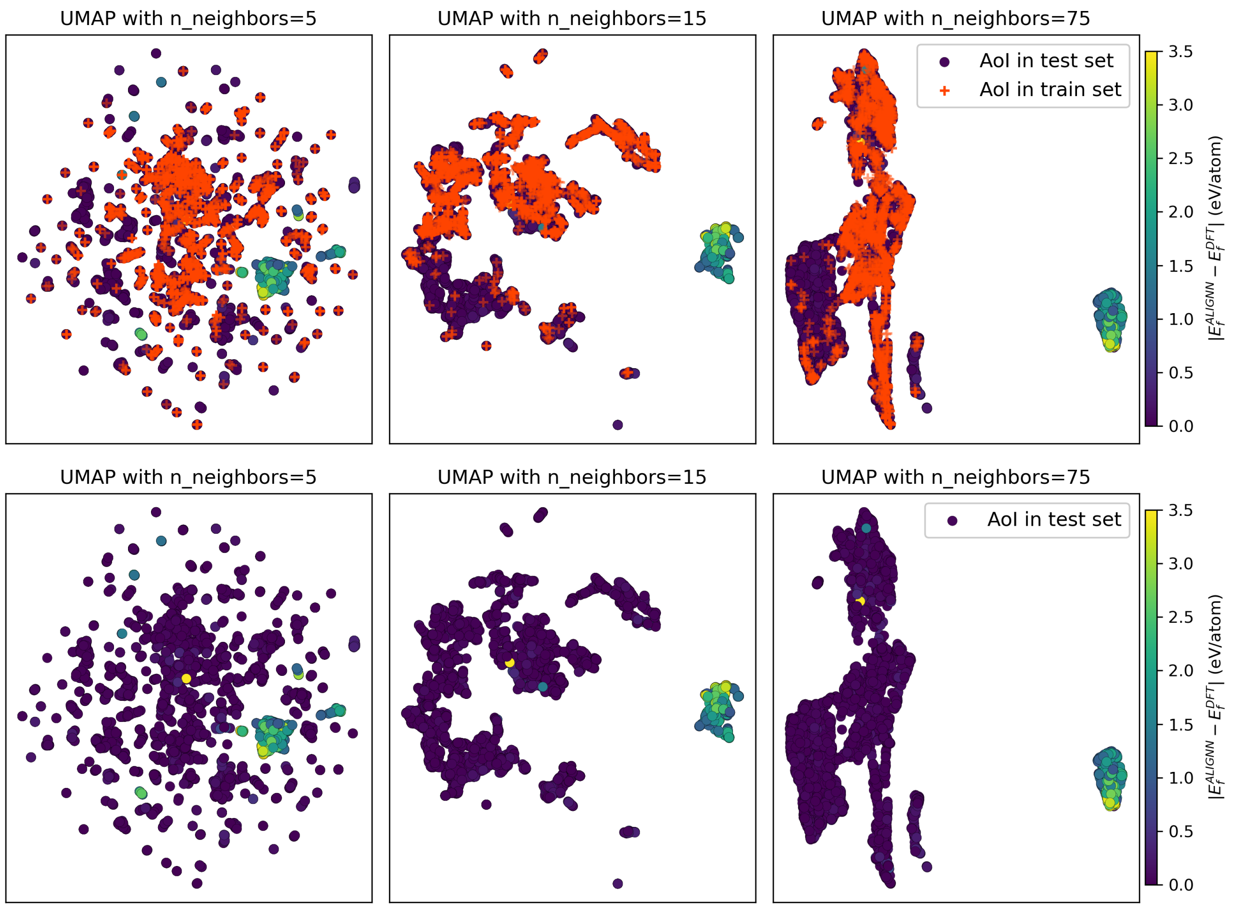


FIG. S4. Two-dimensional UMAP projection (with different values of `n_neighbors`) of the 90-dimensional feature space. The AoI test data are colored by their ALIGNN prediction errors. The AoI training data are shown (hidden) in the upper (lower) panel.
